# Supplementary material for: UDO: Universal Database Optimization using Reinforcement Learning
Source: arXiv:2104.01744 source file (2021-08-26)
Supplement: Supplementary file 1 [file supplementary_proofs.pdf]

# Theoretical Analysis of UDO and Delayed-HOO

## 1. Brief Description of Results

We show, under moderately simplifying assumptions, that UDO converges to optimal configurations. UDO uses an extension of HOO algorithm, which provides this type of guarantee (Theorem 6, (Bubeck et al., 2011)). However, we decompose our search space (into a space for heavy and one for light parameters) and delay evaluation feedback (to amortize reconfiguration costs). In this section, we sketch out our reasoning for why those changes do not prevent convergence.

In doing so, we use regret (Audibert et al., 2007) as the metric of convergence. Given a time horizon $T$, regret $\text{Reg}_T$ is the sum of differences between the performance of the optimal configuration and the configuration achieved by the algorithm at any time step $t \leq T$. If the expected regret of an algorithm grows sublinearly with horizon $T$, it means the algorithm asymptotically converges to optimal configuration as $T \to \infty$.

**Theorem 1 (Regret of HOO (Theorem 6 (Bubeck et al., 2011)))** *If the performance metric $f$ is smooth around the optimal configuration (Assumption 2 in (Bubeck et al., 2011)) and the upper bounds on rewards of all the configurations at depth $h$ are bounded by $c\rho^h$ with $\rho \in (0,1)$ (Assumption 1 in (Bubeck et al., 2011)), expected regret of HOO is*

$$\mathbb{E}[\text{Reg}_T] = O\left(T^{1-\frac{1}{d+2}}(\log T)^{\frac{1}{d+2}}\right) \tag{1}$$

*for a horizon $T > 1$, and $4/c$-near-optimality dimension[1] $d$ of $f$.*

Since a performance metric $f : [a,b]^P \to [a,b] \subset \mathbb{R}$, $d$ is of the same order as the number of parameters $P$. Original HOO uses UCB1 (Auer et al., 2002) rather than UCB-V (Audibert et al., 2007). For brevity of analysis, we follow the same though the proof technique is similar for any UCB-type algorithm.

### 1.1 Regret of Delayed-HOO

Now, we prove that using delayed-UCB1 (Joulani et al., 2013) instead of UCB1 allows us to propose delayed-HOO and also achieves similar convergence properties.

**Theorem 2 (Regret of Delayed-HOO)** *Under the same assumptions as Thm. 1, the expected regret of delayed-HOO is*

$$\mathbb{E}[\text{Reg}_T] = O\left((1+\tau)T^{1-\frac{1}{d+2}}(\log T)^{\frac{1}{d+2}}\right) \tag{2}$$

*for delay $\tau \geq 0$, horizon $T$, and $4/c$-near-optimality dimension $d$ of $f$.*

1. $k$-near-optimality dimension of $f$ is logarithm of the number of $\epsilon$-balls needed to pack a subdomain $C_{k\epsilon}$ of $f$ divided by $\ln(1/\epsilon)$, where $\epsilon \to o$ (Def. 5 in (Bubeck et al., 2011)). It can be seen as growth in metric entropy of the set of $k\epsilon$-optimal configurations w.r.t. $\epsilon$.

©2021 anonymous-author-full-names.

License: CC-BY 4.0, see https://creativecommons.org/licenses/by/4.0/.

**Proof** [Proof Sketch] First, we observe that for delayed-HOO, we can decompose the regret into two terms: one as same as the original HOO and the other one for delay. The first term leads to same result as Eq. (1). Now, the other term is $\sum_{h=1}^{Depth(MCT)} \rho^h (2-d)\tau$. If we follow the same steps as HOO, we obtain this term is $O(\tau T^{1-\frac{2}{d+2}} (\log T)^{\frac{2}{d+2}})$ for $\rho^{Depth(MCT)} = O(T/\log T)$. Thus, we obtain that $\mathbb{E}[R_T(c)] \leq O(((1+\tau) T^{\frac{d+1}{d+2}} (\log T)^{1/(d+2)})$. ■

The bound in Eq. (2) is the same as Eq. (1) with an additional factor $(1+\tau)$, which does not change the convergence in terms of $T$. For delay $\tau = 0$, we retrieve the regret bound of original HOO.

The error in estimated expected reward of any given configuration at time $T$ is

$$\epsilon(T) = \max_c \mathbb{E}[f(c) - \hat{f}_T(c)] = \max_c \frac{1}{T} \mathbb{E}[R_T(c)].$$

Thus, the error $\epsilon(T)$ in estimating the expected performance (or reward) of a configuration using delayed-HOO converges at the rate

$$O\left((1+\tau)\left[\log T/T\right]^{1/(d+2)}\right),$$

where $T$ is the number of times the configuration is evaluated.

### 1.2 Regret of UDO

As we have obtained the error bound of the delayed-HOO algorithm, now we can derive bounds for UDO when using delayed-HOO for heavy and light parameters with two different delays.

**Theorem 3 (Regret of UDO)** *If we use the delayed-HOO as the delayed-MCTS algorithm with delays $\tau$ and $0$, and time-horizons $T_h$ and $T_l$ for heavy and light parameters respectively, the expected regret of UDO us upper bounded by*

$$\mathbb{E}[\mathrm{Reg}_T] = O\left((1+\tau) T^{1-\frac{1}{d+2}} (\epsilon(T_l)^2 \log T)^{\frac{1}{d+2}}\right). \tag{3}$$

*Here, $\epsilon(T_l) = O\left(\left[\log T_l/T_l\right]^{1/(d+2)}\right)$.*

**Proof** [Proof Sketch] The proof for UDO is similar to bounding regret for delayed-HOO on the heavy parameters' configuration space, where the rewards are observed with some estimation error. The estimation error $\epsilon(T_l)$ is unavoidable due to the error in solving light parameter MDP using HOO with no delay. By Theorem 1, $\epsilon(T_l) = O([\log T_l/T_l]^{1/(d+2)})$.

Now, we prove the regret bound in two steps. First, like in the delayed-HOO proof, we decompose the regret of UDO in three error terms due to original HOO, delay-dependent error, and estimation error for light parameters. Then, we plug-in the regret bounds of HOO, delay times suboptimality of expected reward of actions, and bias $\epsilon(T_l)$ induced by HOO as obtained for light parameter MDPs. Now, performing algebraic manipulation leads to the regret bound where the delay factor $(1+\tau)$ and squared error $\epsilon^2(T_l)$ appear as multiplicative factors. ■

Thus, deviation in the expected performance of the configuration returned by UDO from the optimal one is $O\left((1+\tau)\left[\frac{\epsilon^2(T_l)\log T_h}{T_h}\right]^{1/(d+2)}\right)$. Here, $T_h$ and $T_l$ are the number of steps allotted for the heavy and light parameters respectively. The deviation in performance of the configuration selected by UDO vanishes as $T_h, T_l \to \infty$.

## 2. Details of Theoretical Analysis

### 2.1 Assumptions

In order to proof convergence of UDO, we have to oblige by the assumptions regarding theoretical analysis of HOO (Bubeck et al., 2011). In this section, we elaborate them.

In any MCTS algorithm with a UCB-type selection algorithm, we grow a tree such that each node represents a configuration $c$, and the corresponding upper confidence intervals partition the domain of the performance metric $f$. As the Monte Carlo tree grows, we obtain a hierarchical partitioning of the domain. As we want the confidence intervals to shrink with increase in their depth, we need to ensure certain regularity of such hierarchical partition. Assumption 1 quantifies and bounds this desired regularity criterion.

Let us represent the tree covering the domain as $(X_{h,i})_{h,i=0,1}^{H,2^h}$, where $X_{h,i}$ is the interval covered by the $i$-th node at depth $h$. The specific value obtained at that node is denoted as $x_{h,i}$. Let us also assume that the domain of $f$, say $\mathcal{X} \subset \mathbb{R}^D$, has a dissimilarity measure $l$ that can quantify difference between two inputs.

**Assumption 1 (Hierarchical Partition with Decreasing Diameter and Shape)**

*1.1* Decreasing diameters. *There exists a decreasing sequence $\delta(h) > 0$ such that*

$$\operatorname{diam}(X_{h,i}) \triangleq \max_{x \in X_{h,i}} l(x_{h,i}, x) \leq \delta(h), \tag{4}$$

*for any depth $h \geq 0$, for any interval $X_{h,i}$, and for all $i = 1, \ldots, 2^h$. For simplicity, we consider that $\delta(h) = \rho^h$ for some $\rho \in (0,1)$.*

*1.2* Regularity of the intervals. *There exists a constant $c > 0$ such that for any depth $h \geq 0$, every interval $X_{h,i}$ contains at least a ball $\mathcal{B}_{h,i}$ of radius $c\rho^h$ and center $x_{h,i}$ in it. Since the tree creates a partition at any given depth $h$, $\mathcal{B}_{h,i} \cap \mathcal{B}_{h,i} = \emptyset$ for all $1 \leq i < j \leq 2^h$.*

The other condition that we need to prove convergence of HOO to a global optimum is smoothness of $f$ around the optimum, say $x^*$. This is often referred as weak Lipschitz property.

**Assumption 2 (Weak Lipschitzness of $f$)** *For all $x, y \in \mathcal{X}$, $f$ satisfies*

$$f^* - f(y) \leq f^* - f(x) + \max\{f^* - f(x), l(x,y)\}, \tag{5}$$

*where $f^*$ is the optimal value of $f$ achieved at a global optimum $x^*$.*

This assumption holds true if
1. either $f(x) - f(y) \leq l(x, y)$ and $f^* - f(x) \leq \max_y l(x, y)$,
2. or $f(x) - f(y) \leq f^* - f(x)$ and $f^* - f(x) \geq \max_y l(x, y)$.

This property basically implies that there is no sudden drop or jump in performance $f$ for configurations around the optimal configuration $c^*$. Weak Lipschitzness can hold even for discontinuous functions. Thus, it widens applicability of HOO's analysis to more general performance metrics and configuration spaces in comparison with algorithms that explicitly need gradients or smoothness in some form.

## 2.2 Background: Definitions and Results

### 2.2.1 Near-optimality Dimension

Let us denote the set of $\epsilon$-optimal states as

$$\mathcal{X}_\epsilon \triangleq \{x \in \mathcal{X} | f(x) \geq f^* - \epsilon\}.$$

Near-optimality dimension quantifies the number of $l$-balls needed to pack this set of $\epsilon$-optimal states. First, we define the $l$-ball.

**Definition 4 ($l$-ball)** *An $l$-ball of radius $\rho$ is $\mathcal{B}_\rho \triangleq \{x | \max_y l(x, y) \leq \rho \ \forall \ x, y \in \mathcal{B}_\rho \subseteq \mathcal{X}\}$.*

Now, we define the $c$-near-optimality dimension.

**Definition 5 ($c$-near-optimality dimension)** *$c$-near-optimality dimension is the smallest $d \geq 0$, such that for all $\epsilon > 0$, the maximal number of disjoint $l$-balls of radius $c\epsilon$ whose centres can be accommodated in $\mathcal{X}_\epsilon$ is $O(\epsilon^{-d})$.*

This is a joint property of the performance metric $f$ and dissimilarity measure $l$. $d$ is independent of the MCTS algorithm of choice.

### 2.2.2 Regret

Typically, in a multi-armed bandit problem, an algorithm encounters $k$ unknown probability distributions of rewards. The algorithm can only known more about it by sampling the distribution (or often referred as *arm*). Now, the goal of a bandit algorithm is to maximise total sum of accumulated rewards, i.e. $\sum_{t=1}^{T} R_t$, given a time horizon $T$. Typically, what we aim to maximize is the expectation of accumulated rewards, i.e. $\mathbb{E}[\sum_{t=1}^{T} R_t]$.

If we want to maximize the value of a configuration $c$ situated at a node $(h, i)$ of the tree, it becomes equivalent to maximising the total obtained reward through its next $T$ children. Thus, multi-armed bandit algorithms are deployed in MCTS in order to maximize the value of a configuration.

There is an alternative way of formulating the goal of a bandit, i.e. minimizing deviation of the expected accumulated reward $\mathbb{E}[\sum_{t=1}^{T} R_t]$ from the maximal achievable reward $Tf^*$.

This is called *expected cumulative regret* or simply *regret.*

$$\begin{aligned}
\mathbb{E}[\mathrm{Reg}_T] &= T\mu^* - \sum_{a=1}^{K} \mathbb{E}_\pi \left[N_T^a\right] \mu_a \\
&= \sum_{a=1}^{K} \mathbb{E}_\pi \left[N_T^a\right] (\mu^* - \mu_a) \qquad \left(\text{since, } T = \sum_{a=1}^{K} \mathbb{E}_\pi \left[N_T^a\right]\right) \\
&= \sum_{a=1}^{K} \text{Expected \# decision } a \text{ is taken} \times \text{ Expected suboptimality of arm } a
\end{aligned}$$

Following the traditional analysis of MCTS algorithms (Munos, 2014), we are going to use regret of an MCTS algorithm as its measure of performance. Less is the regret better is the performance of an MCTS algorithm. If the upper bound on regret grows sublinearly with horizon $T$, it means that the error incurred by corresponding algorithm asymptotically vanishes.

The other performance metric relevant to MCTS algorithm is the expected deviation, or *error*, incurred at any time $t$:

$$r_t = \max_x f(x) - f(x_t) = f^* - f(x_t). \tag{6}$$

$r_t$ is also termed as *simple regret.* This metric is different than regret but in case of HOO, their expected values are closely related. If we choose the state $x_t$ uniformly randomly from all the states observed till time $T$, the expected value of error (or simple regret) becomes

$$\mathbb{E}[r_t] = \mathbb{E}[f^* - f(x_t)] = \frac{1}{T}\sum_{i=1}^{t}[f^* - f(x_i)] = \frac{1}{T}\mathrm{Reg}_T \tag{7}$$

Later, we will use this relation to convert the traditional regret bound originating from the bandit algorithms used in MCTS to the expected estimation error achieved by corresponding MCTS algorithm.

#### 2.2.3 Regret of HOO

After elaborating all the required assumptions and definitions, and choosing regret as our primary performance measure, we now state the regret bound of original HOO algorithm (Theorem 6 (Bubeck et al., 2011)).

**Theorem 6 (Regret of HOO)** *If Assumptions 1 and 2 hold true, expected regret of HOO*

$$\mathbb{E}[\mathrm{Reg}_T] = O\left(T^{1-\frac{1}{d+2}}(\log T)^{\frac{1}{d+2}}\right) \tag{8}$$

*for a horizon $T > 1$, and $4/c$-near-optimality dimension $d$ of $f$.*

Hereafter, we refer to the term $T^{-1/(d+2)}(\log T)^{1/(d+2)}$ as $\mathrm{HOO}(T)$. Thus, for the original HOO algorithm, we get that $\mathbb{E}[\mathrm{Reg}_T] = O\left(T\ \mathrm{HOO}(T)\right)$ and $\mathbb{E}[r_T] = O\left(\mathrm{HOO}(T)\right)$.

### 2.3 Regret of Delayed-HOO

### 2.4 Regret of UDO

## References

J.-Y. Audibert, R. Munos, and C. Szepesvári. Tuning bandit algorithms in stochastic environments. In M. Hutter, R. A. Servedio, and E. Takimoto, editors, *Algorithmic Learning Theory*, pages 150–165, Berlin, Heidelberg, 2007. Springer Berlin Heidelberg.

P. Auer, N. Cesa-bianchi, and P. Fischer. Finite time analysis of the multiarmed bandit problem. *Machine Learning*, 47(2-3):235–256, 2002.

S. Bubeck, R. Munos, G. Stoltz, and C. Szepesvári. X-armed bandits. *Journal of Machine Learning Research*, 12(5), 2011.

P. Joulani, A. György, and C. Szepesvari. Online learning under delayed feedback. *30th International Conference on Machine Learning, ICML 2013*, (PART 3):2503–2511, 2013. doi: 10.14288/1.0044651.

R. Munos. From bandits to Monte-Carlo tree search: The optimistic principle applied to optimization and planning. *Foundations and Trends in Machine Learning*, 7(1):1–129, 2014. ISSN 19358237. doi: 10.1561/2200000038.
